# Supplementary material for: Holographic Algorithms with Matchgates Capture Precisely Tractable Planar #CSP
Source: arXiv:1008.0683 source file (2010-08-04)
Supplement: Supplementary file 1 [file appendix.tex]

\section*{Appendix}
\begin{lemma}
Pl-Holant$^c([0,0,1,0,0])$ is \#P-hard.
\end{lemma}

\begin{lemma}\label{lemma:010x}
If $a \not \in \{-1,0,1\}$, we can interpolate all $[0,1,0,x]$ starting from $[0,1,0,a]$.
\end{lemma}

\begin{proof}
Our start point here is that ${\rm Holant} ([0,1,0,0])$ is \#P-hard.
This is exactly the perfect matching problem in 3-regular graph
\cite{DagumL92}. So the problem is \#P-hard if $a=0$.

Now assume that $a \not \in \{-1,0,1\}$, and we use this signature
to interpolate all the signature of form $[0,1,0,x]$, in particular,
we can interpolate $[0,1,0,0]$ and finish the hardness reduction.

\begin{figure}[htbp]
\begin{center}
\epsfxsize=4 in \epsffile{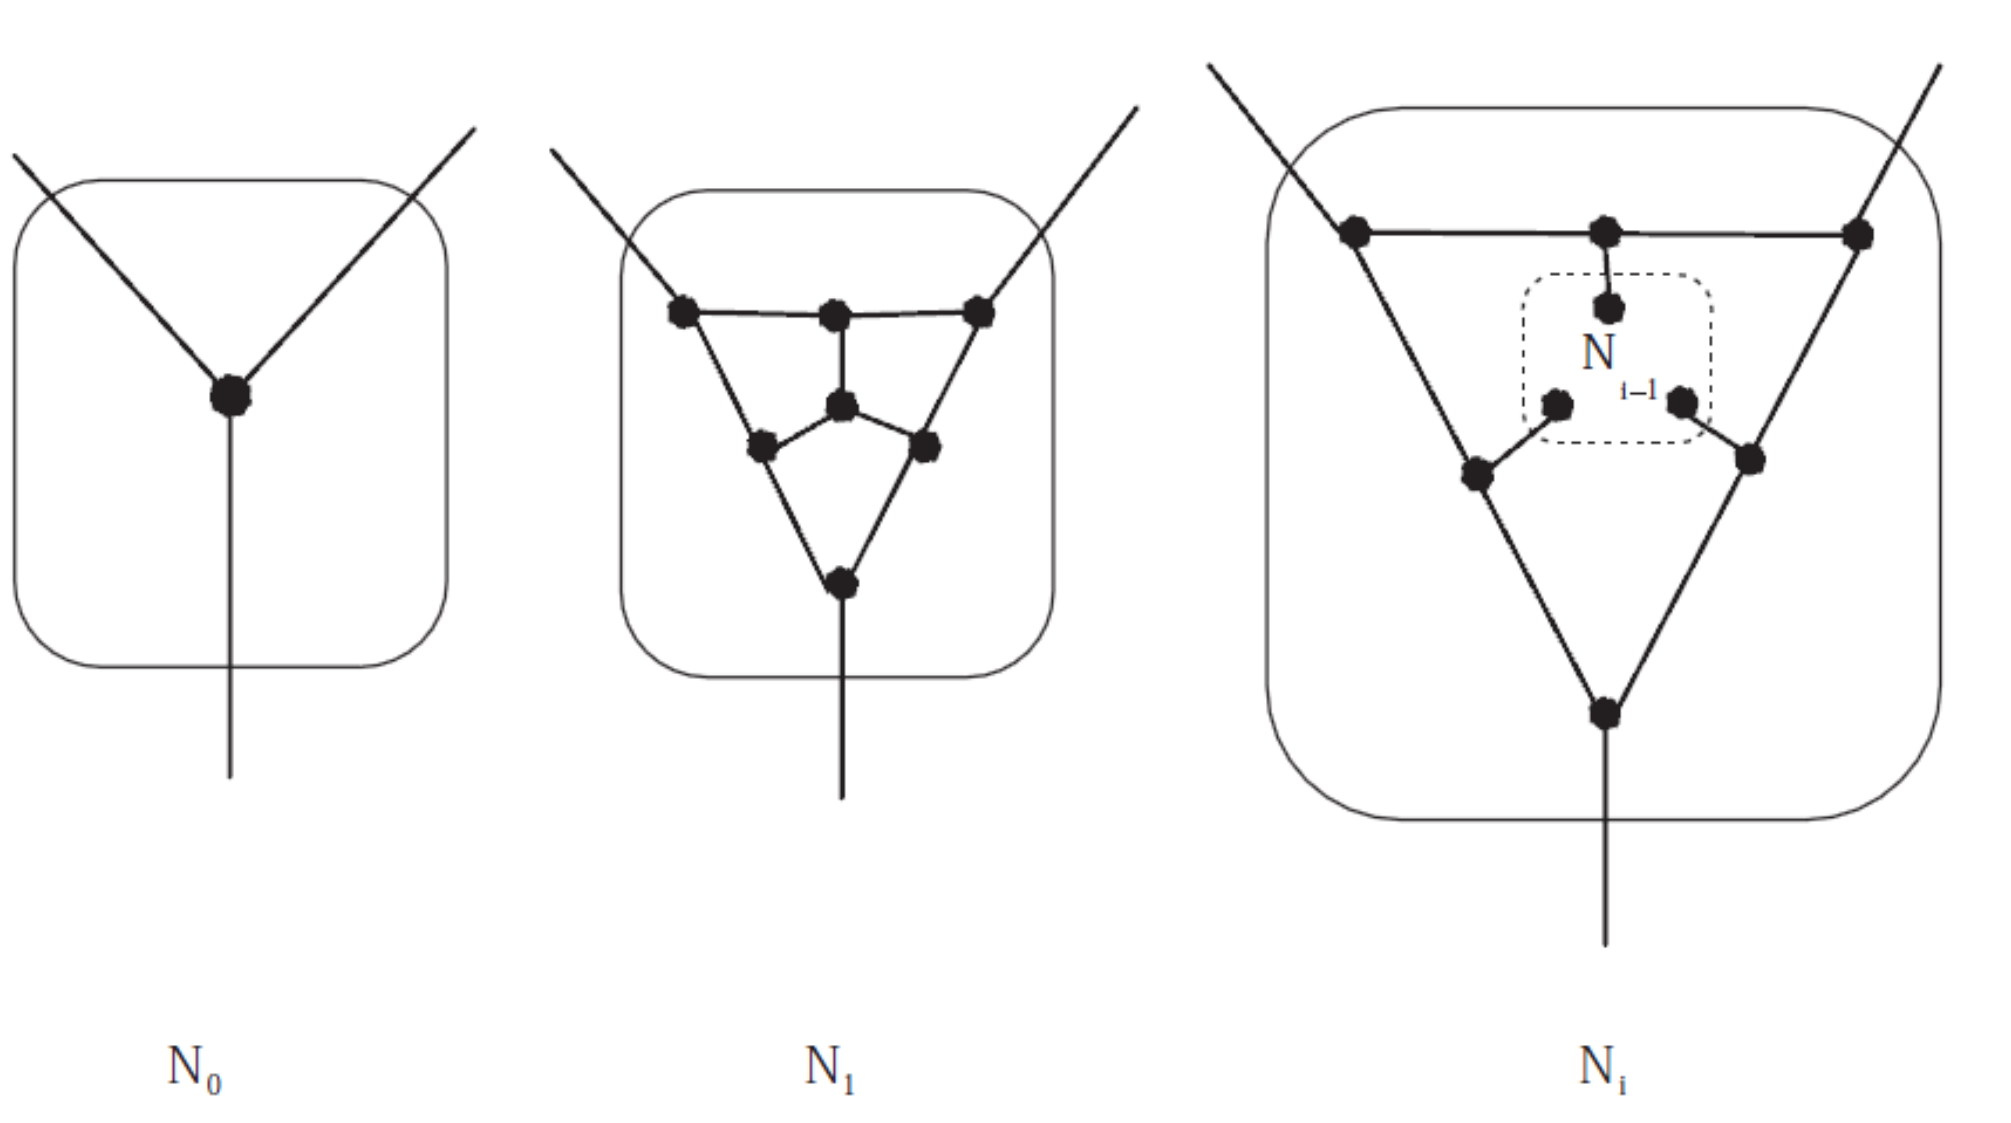} \caption{The recursive
construction. The signature of every vertex in the gadget is
$[0,1,0,a]$. } \label{Figure:010x}
\end{center}
\end{figure}

The recursive construction is depicted by Figure \ref{Figure:010x}.
By a simple parity argument, every \FF  ~$N_i$ has a signature of
the form $[0,x_i,0,y_i]$. After some calculation, we can get that
they satisfy the following recursive relation:
\[\begin{bmatrix}x_{i+1} \\ y_{i+1} \end{bmatrix}=
\begin{bmatrix}3(a^2+1) & a^3+a \\ 3(a^3+a) & a^6+1 \end{bmatrix}
\begin{bmatrix}x_{i} \\ y_{i} \end{bmatrix}.\]
%%Pinyan: Please double check it.
In this case, the signature we want to interpolate are of arity $3$.
But since all of them are of form $[0,x_i,0,y_i]$ with two
dimensions freedom. We can also use the interpolation method as in
Section \ref{sec:interpolation}. Let $A=\begin{bmatrix}3(a^2+1) &
(a^3+a) \\ 3(a^3+a) & a^6+1
\end{bmatrix}$, then $(A, [1,a]^{\rm T})$ forms a recursive
construction. Since ${\rm det}(A)=3(a^4-1)^2\neq 0$, the first
condition holds. Its characterize equation is $X^2-(a^6+3 a^2+4)X
+3(a^4-1)^2=0$. For this quadratic equation, $\Delta=(a^6-3 a^2
-2)^2+ 12 (a+a^3)^2 >0$. So $A$ has two distinct real eigenvalues.
The sum of the two eigenvalues is $a^6+3 a^2+4$ which is larger than
zero. So they are not opposite to each other. Therefore, the ratio
of these two eigenvalues is not a root of unity and the third
condition holds. Consider the second condition, if the initial
vector $[1,a]$ is a column eigenvectors of $A$. We have
$A\begin{bmatrix}1
\\ a
\end{bmatrix}= \lambda \begin{bmatrix}1 \\ a
\end{bmatrix} $, where $\lambda$ is one eigenvalue of $A$. From
this, we will conclude that $a(a^2-1)(a^4-1)=0$,
%$a^-1=0$
which will not happen given $a \not \in \{-1,0,1\}$. To sum up, this
recursive relation satisfies all the three conditions of Lemma
\ref{lemma:interpolation_conditions} and can be used to interpolate
all the signatures of form $[0,1,0,x]$. This completes the proof.
\end{proof}

\begin{lemma}\label{lemma:inG1F2G3}
If ${\cal F} \not \subseteq {\cal G}_1 \cup {\cal F}_2\cup {\cal
G}_3$, then Theorem \ref{thm:holant-c} holds.
\end{lemma}

\begin{proof}
If ${\cal F} \not \subseteq {\cal G}_1 \cup {\cal G}_2\cup {\cal
G}_3$, then by Lemma \ref{lemma:inG1G2G3}, we are done. Otherwise,
there exists a signature $f \in {\cal F} \subseteq {\cal G}_1 \cup
{\cal G}_2\cup {\cal G}_3 $ and $f \not \in {\cal G}_1 \cup {\cal
F}_2\cup {\cal G}_3$. Then it must be the case that $f \in {\cal
G}_2$. Note that every signature with arity less than $3$ in ${\cal
G}_2$ is also contained in ${\cal G}_1 \cup  {\cal G}_3$, so $f$ is
of arity larger than $2$. Since $f \not \in {\cal G}_1$, there is
some non-zero in the middle of the signature $f$, after
normalization, we can assume there is a sub signature of form
$[0,1,0,x]$ (or $[x,0,1,0]$). If $x\neq \pm 1$, then by Lemma
\ref{lemma:010x}, we know the problem is \#P-hard and we are done.
Otherwise, for every such pattern , we have $x=\pm 1$. Since $f \not
\in {\cal F}_2$, then there is some sub signature $[0,1,0,-1]$ and
because $f \not \in {\cal G}_3$, there is some sub signature
$[0,1,0,1]$. Therefore, there is a sub signature $[1,0,1,0,-1]$ of
$f$. Then we can construct  a \FF  ~as Figure \ref{Figure:1010-1} ,
%\begin{figure}[htbp]
%\begin{center}
%\epsfxsize=2 in \epsffile{gate_1010-1.eps} \caption{ The signature
%of every degree $4$ vertex in the gadget is  $[1,0,1,0,-1]$. And the
%signature of the degree $1$ vertex in the gadget is  $[1,0]$. }
%\label{Figure:1010-1}
%\end{center}
%\end{figure}
whose signature is $[8,0,4,0]$. So by Lemma \ref{lemma:010x}, we
know that the problem is \#P-hard and we are done. This completes
the proof.
\end{proof}

\begin{lemma}\label{lemma:inG1G3}
If ${\cal F} \not \subseteq {\cal G}_1 \cup  {\cal G}_3$, then
Theorem \ref{thm:holant-c} holds.
\end{lemma}

\begin{proof}
If ${\cal F} \not \subseteq {\cal G}_1 \cup {\cal F}_2\cup {\cal
G}_3$, then by Lemma \ref{lemma:inG1F2G3}, we are done. Otherwise,
there exists a signature $f \in {\cal F} \subseteq {\cal G}_1 \cup
{\cal F}_2\cup {\cal G}_3 $ and $f \not \in {\cal G}_1 \cup {\cal
G}_3$. Then it must be the case that $f \in {\cal F}_2$. Note that
every signature with arity less than $3$ in ${\cal F}_2$ is also
contained in ${\cal G}_1 \cup  {\cal G}_3$, so $f$ is of arity
larger than $2$. Then $f$ has a sub signature $[1,0,1,0]$ or
$[0,1,0,1]$. By symmetry, we assume it is $[1,0,1,0]$. If ${\cal F}
\subseteq {\cal F}_1 \cup {\cal F}_2 \cup {\cal F}_3 $, then Theorem
\ref{thm:holant-c} trivially holds and there is nothing to prove. If
not, there exists a signature $g$ is in ${\cal G}_1-{\cal F}_1 \cup
{\cal F}_2 \cup {\cal F}_3 ~(\subseteq{\cal G}_1-{\cal F}_1)$ or
${\cal G}_3-{\cal F}_1 \cup {\cal F}_2 \cup {\cal F}_3
~(\subseteq{\cal G}_3-{\cal F}_3)$.

For the first case,  $g \in ({\cal G}_1-{\cal F}_1)$, then after a
scale, $g$ is of form $[1,0,0,\cdots, b]$, where $b \not \in
\{-1,0,1\}$. If the arity of $g$ is odd, we can realize $[1,b]$. (We
connect its every two dangling edges into one edge and left one
dangling edge.) Then connecting this unary signature to one dangling
edge of $[1,0,1,0]$,
 we can realize a binary
signature $[1,b,1]$.
% by a ${\cal F}$-gate as in Fig \ref{}.
Then by Lemma \ref{lemma:interpolation}, Theorem \ref{thm:holant-c}
holds. If the arity of $g$ is even, we can realize $[1,0,b]$ (left
two dangling edges). By connecting  one of its dangling edge to one
dangling edge of $[1,0,1,0]$, we can have a new ternary signature
$[1,0,b,0]$.
% by a ${\cal F}$-gate as in Fig \ref{}.
By lemma \ref{lemma:010x}, we know the problem is \#P-hard.

For the second case $g \in ({\cal G}_3-{\cal F}_3)$, then $g$ has a
sub signature of form $[1,b]$, where $b \not \in \{-1,0,1\}$. By the
same argument as above, Theorem \ref{thm:holant-c} holds. This
completes the proof.
\end{proof}

%\begin{lemma}
%If $[1,0,1,0] \in {\cal F} $ or $[0,1,0,1] \in {\cal F} $, then Theorem \ref{thm:holant-c} holds.
%\end{lemma}
%
%\begin{lemma}
%If $[1,\lambda] \in {\cal F} $, where $\lambda \not \in \{-1,0,1\}$, then Theorem \ref{thm:holant-c} holds.
%\end{lemma}

\begin{lemma}\label{lemma:inG1F3}
If ${\cal F} \not \subseteq {\cal G}_1 \cup  {\cal F}_3$, then
Theorem \ref{thm:holant-c} holds.
\end{lemma}

\begin{proof}
If ${\cal F} \not \subseteq {\cal G}_1 \cup {\cal G}_3$, then by
Lemma \ref{lemma:inG1G3}, we are done. Otherwise, there exists a
signature $f \in {\cal F} \subseteq {\cal G}_1 \cup {\cal G}_3 $ and
$f \not \in {\cal G}_1 \cup {\cal F}_3$. Then it must be the case
that $f \in {\cal G}_3$ , and $f$ has a sub signature of form
$[1,a,-1]$, where $a \not \in \{-1,0,1\}$.
%XMJ: the length of this sub-signature is 3,
%because all signatures of length 2 are in G_1.
%because $f \not \in {\cal F}_3$, $a \not \in \{-1,0,1\}$.

If ${\cal F}  \subseteq (\{[1,0,1] \} \cup  {\cal G}_3)$, then ${\rm
Holant}^* ({\cal F})$  is polynomial time computable by Theorem
\ref{thm:main} and as a result Theorem \ref{thm:holant-c} trivially
holds and there is nothing to prove.

If not, there exists a signature $g \in {\cal F}  \subseteq {\cal
G}_1 \cup  {\cal G}_3$ and $g \not \in \{[1,0,1] \} \cup  {\cal
G}_3$. Then it mush be the case that $g \in {\cal G}_1$. The arity
of $g$ is large than $1$. %,because G_3 contains all functions of arity 1.

%\begin{figure}[htbp]
%\begin{center}
%\epsfxsize=2 in \epsffile{gata_for_lemma2.6.eps} \caption{The
%function on degree 2 nodes is $[1,a,-1]$, and the function on degree
%3 nodes is $[1,0,0,b]$. } \label{Figure:[1,a^2b,b^2]}
%\end{center}
%\end{figure}
gate_1_a2b_b2

If the arity of $g$ is $2$, then $g$ is of form $[1,0,b]$, where $b
\not \in \{-1,0,1\}$. Connecting two signatures $[1,0,b]$ to the
both sides of one binary signature $[1,a,-1]$, we can get a new
binary signature $[1,ab, -b^2]$. It satisfies all the conditions of
Lemma \ref{lemma:interpolation}, and we are done. If the arity of
$g$ is larger than $2$, then we can always realize a signature
$[1,0,0,b]$, where $b\neq 0$. (We connect the unary signature
$[1,a]$ to all its dangling edges except the three ones.)
 Then we can use an \FF ~as Figure \ref{Figure:[1,a^2b,b^2]}.
Its signature is $[1,a^2b, b^2]$, and by Lemma
\ref{lemma:interpolation}, we are done. This completes the proof.
\end{proof}

By the above lemmas, the only case we have to handle is that ${\cal
F} \subseteq {\cal G}_1 \cup  {\cal F}_3$. This is done by the
following lemma. which completes the proof of Theorem
\ref{thm:holant-c}.

\begin{lemma}\label{lemma:G1F3}
If ${\cal F}  \subseteq {\cal G}_1 \cup  {\cal F}_3$, then Theorem
\ref{thm:holant-c} holds.
\end{lemma}

\begin{proof}
If ${\cal F} \subseteq {\cal F}_1 \cup {\cal F}_3$ or ${\cal
F}\subseteq {\cal U} \cup {\cal F}_3 \cup \{[1,0,1]\}$, then ${\rm
Holant}^c({\cal F})$ is computable in polynomial time and
Theorem\ref{thm:holant-c} holds. Otherwise, there are two cases.
There exists $f\in {\cal F} $ such that $f \in {\cal G}_1$ but $f
\not \in{\cal F}_1 \cup {\cal U} \cup {\cal F}_3 $. So the arity of
$f$ is larger than $1$. W.l.o.g, we can assume $f$ has form
$[1,0,a]$ or $[1,0,0,a]$, where $a \not \in \{-1,0,1\}$. (By
connecting its dangling edges together except two or three depends
on the parity of the arity of $f$. ) The other case is that there
exists $f_1, f_2\in {\cal G}_1$ such that $f_1 \in {\cal F}_1$ but
$f_1 \not \in{\cal U} \cup {\cal F}_3 \cup \{[1,0,1]\}$, and $f_2
\in {\cal U}$ but $f_2 \not \in {\cal F}_1$. So the arity of $f_1$
is larger than $2$ and with form $[1,0,0,\cdots,\pm 1]$, and $f_2$
is of form $[1,a']$, where $a' \not \in \{-1,0,1\}$. By connecting
all the dangling edges of $f_1$ except two with $f_2$, we can
construct a \FF ~with signature of form $[1,0,a]$, where $a \not \in
\{-1,0,1\}$.This is one of the above two forms.

If ${\cal F}  \subseteq {\cal G}_1 \cup  \{[0,1,0]\}$, then
 ${\rm Holant}^c
({\cal F})$ is computable in polynomial time and Theorem
\ref{thm:holant-c} holds. Otherwise, there exists $g\in {\cal F}
\subseteq {\cal G}_1 \cup  {\cal F}_3 $, and $g \not \in {\cal G}_1
\cup  \{[0,1,0]\}$. Then $g$ must have one of the following sub
signatures: $[1,1,-1],[1,-1,-1],[1,0,-1,0],[0,1,0,-1]$. By
symmetric, we only need to consider two cases $[1,1,-1]$ and
$[1,0,-1,0]$.
%Right. When "symmetric", f=[1,0,a], will turn into [a,0,1]=a[1,0,1/a], 1/a \not \in \{-1,0,1\} either.

According to $f$ and $g$, we have four cases. If $f=[1,0,a]$ and
$g=[1,1,-1]$, then connecting them together into a chain $fgf$, we
can realize $[1,a,-a^2]$. By Lemma \ref{lemma:interpolation}, we are
done. If $f=[1,0,a]$ and $g=[1,0,-1,0]$, for each of dangling edges
of $g$, we extend it by one copy of $f$. Then we can realize
$[1,0,-a^2,0]$. So by lemma \ref{lemma:010x}, the problem is
\#P-hard. If $f=[1,0,0, a]$ and $g=[1,1,-1]$, we can connect a unary
signature $[1,1]$ (sub signature of $g$) to one dangling edge of
$f$, and realize a binary signature $f=[1,0,a]$. This reduce to the
first case, which has been proved. If $f=[1,0,0,a]$ and
$g=[1,0,-1,0]$, we can realize a unary signature $[1,a]$ from $f$
and then connect this unary signature to one dangling edge of $g$ to
realize $[1,-a,-1]$. Note that $[1,-a,-1]\not \in {\cal G}_1 \cup
{\cal F}_3$, by Lemma \ref{lemma:inG1F3}, we are done.
\end{proof}
